# Supplementary material for: AugInsert: Learning Robust Visual-Force Policies via Data Augmentation for Object Assembly Tasks
Source: arXiv:2410.14968 source file (2025-08-01)
Supplement: Supplementary file 1 [file appendix.tex]

\subsection{Task Variation Details}

In this section, we provide more explicit details on the formulation and implementation of our task variations in simulation.

\begin{enumerate} [leftmargin=*]
    \item \textbf{\textit{Peg and Hole Shape:}} The 9 possible peg and hole shapes are key, cross, diamond, line, circle, pentagon, hexagon, key, and u. The intrusions are built with a 5mm uniform tolerance on all sides.
    \item \textbf{\textit{Object Body Shape:}} The 3 possible object body shapes are cube (7.6cm on all sides), cylinder (7.6cm height and diameter), and octagonal prism (7.6cm height and diameter). The thin versions of these objects for the peg shape have $60\%$ the width of the full-sized shapes.
    \item \textbf{\textit{Grasp Pose:}} X-axis translation variations lie within a distance of [-1.7cm, 1.7cm] from the center of the object face (these offsets are scaled down to $60\%$ for thin object body shapes). Z-axis translation variations lie within a distance of [0.0cm, 1.4cm] from the center of the object face. Y-axis rotation variations range from [-10.0$\degree$, 10.0$\degree$], and Z-axis rotation variations are sampled from \{0$\degree$, 90$\degree$, 270$\degree$\} (180$\degree$ was left out due to simulation instability).
    \item \textbf{\textit{Scene Appearance:}} Lighting variations involve both lighting color and the status of the light (either on or off). Object colors are sampled uniformly from all possible colors in the Robosuite \cite{zhu2020robosuite} simulation, and floor textures were sampled from a discrete set of 20 possible textures (6 for training and 14 for evaluation).
    \item \textbf{\textit{Camera Pose:}} Camera position is perturbed in the range of [-4cm, 4cm] on the x, y, and z axes, and camera rotation is perturbed by sampling a random axis-angle rotation (with the axis sampled from a normalized spherical Gaussian and the angle sampled from [0$\degree$, 10$\degree$]) and applying it to the camera's base orientation.
    \item \textbf{\textit{Sensor Noise:}} For force-torque readings, zero-mean Gaussian noise is applied to forces and torques separately (with a standard deviation of 5N for force and 0.15N-m for torque). For proprioceptive readings, zero-mean Gaussian noise is applied to end-effector position and orientation separately (with a standard deviation of 0.1cm for position and 0.57$\degree$ for orientation).
\end{enumerate}

\subsection{Model Architecture}

\begin{figure*}[h!]
     \centering
     \includegraphics[width=0.9\textwidth]{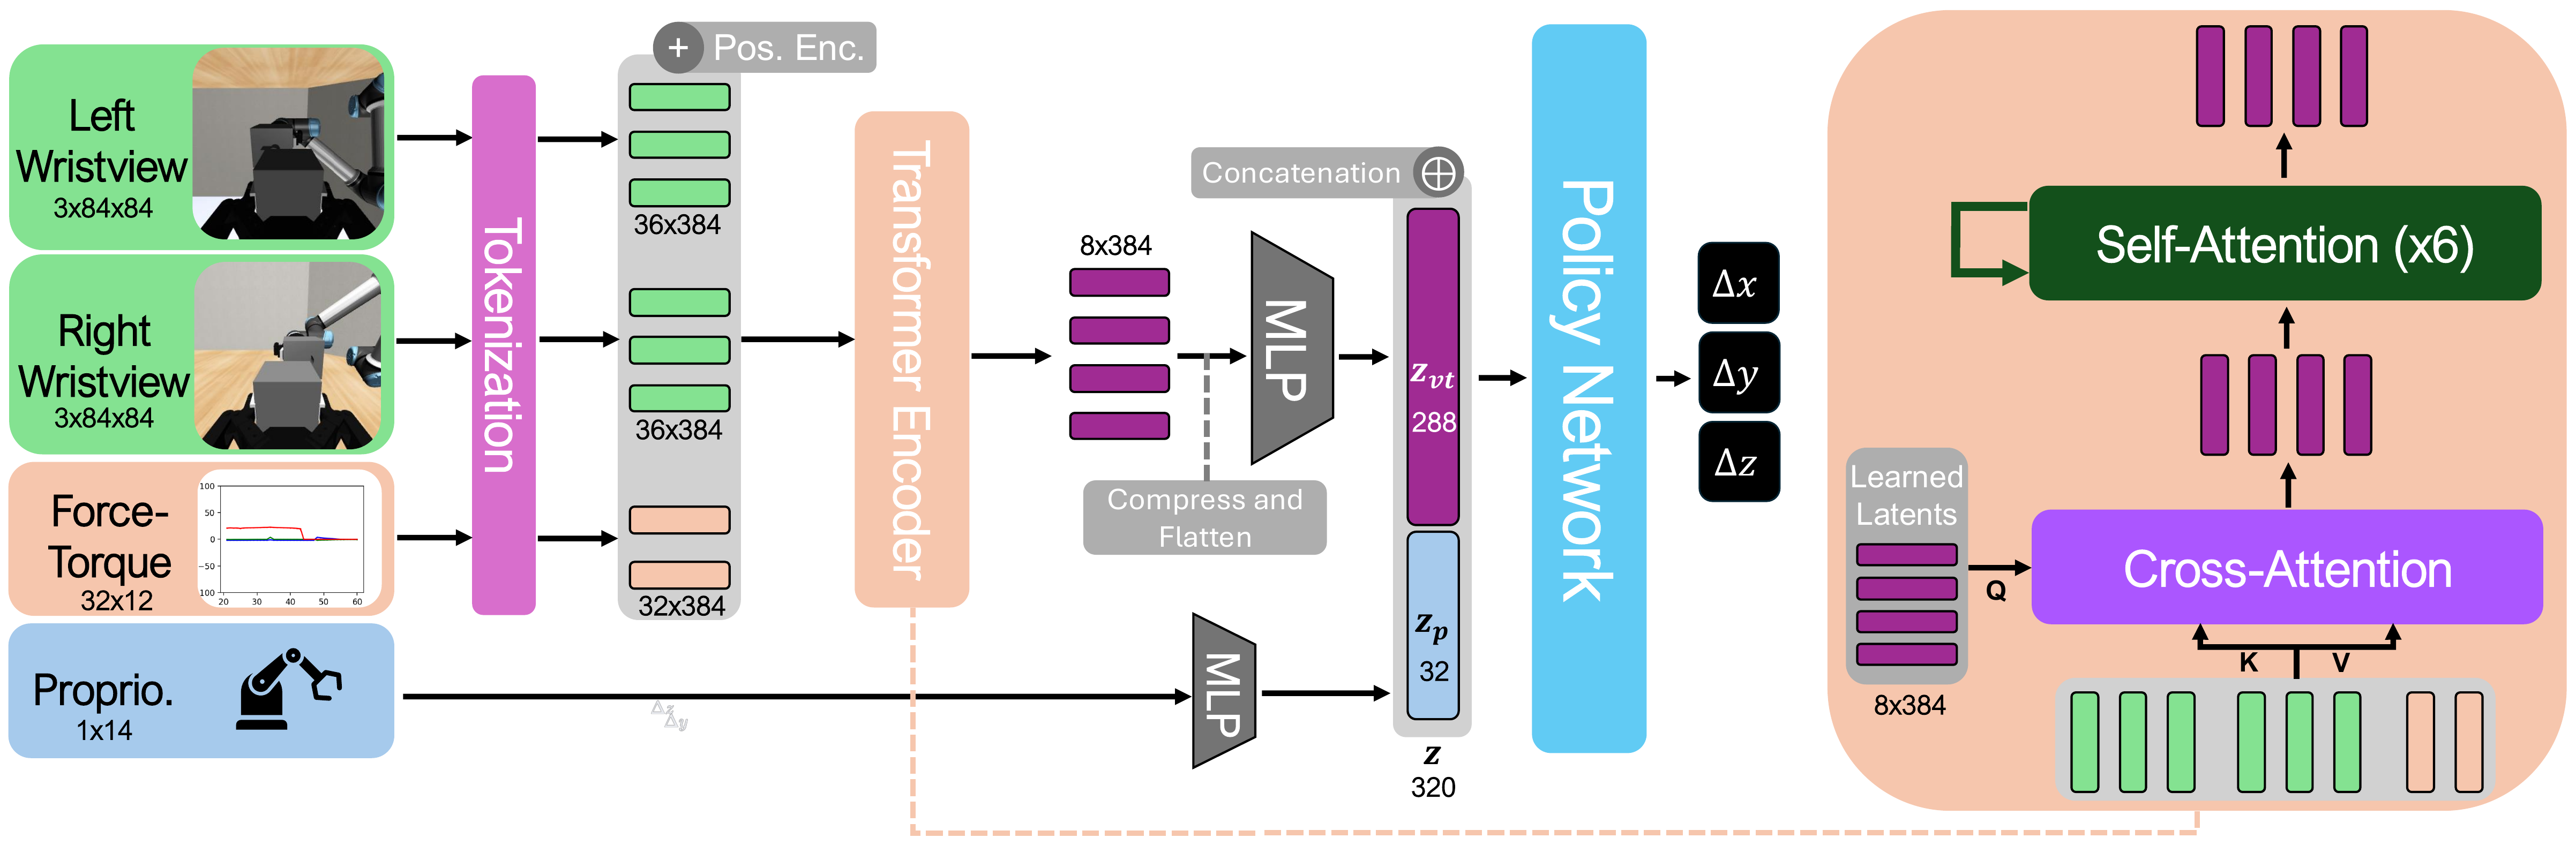}
     \caption{\footnotesize{An extended view of our network architecture with added component dimensions and a visualization of our visuotactile transformer encoder.}}
     \label{fig:extended-architecture}
\end{figure*}

In this section, we provide further details for our observation encoder and policy network architectures, an extended version of which can be found in Figure \ref{fig:extended-architecture}.

To encode our observations, we draw upon the success of visuotactile transformer encoders \cite{chen2023visuo} and utilize a similar attention-based mechanism for RGB and tactile modality fusion. Rather than performing self-attention directly with the input tokens, we found that introducing a cross-attention step similar to the PerceiverIO \cite{jaegle2021perceiver, jaegle2022perceiverio} architecture seemed to work best for our task. The PerceiverIO module has been used in other robotic manipulation contexts \cite{shridhar2023peract} to encode high-dimensional data while still maintaining a high-quality representation.

We tokenize our inputs by computing linear projections of both visual patches \cite{dosovitskiy2021an} for RGB inputs and individual readings per timestep for the force-torque input, and then add modality-specific position encodings. We then cross-attend these input tokens with a set of 8 learned latent vectors that then travel through a series of self-attention layers before ultimately being compressed and projected (as in \cite{chen2023visuo}) to an output latent embedding $z_{vt} \in \mathbb{R}^{288}$. We encode proprioception with a multilayer perceptron to get an output embedding $z_{p} \in \mathbb{R}^{32}$ and concatenate $z_{vt}$ and $z_p$ to get $z \in \mathbb{R}^{320}$, which is used as input to the policy network. The policy network is then a multilayer perceptron that outputs 3-dimensional actions $a \in \mathcal{A}$ that represent end-effector position deltas for one of the arms.

\subsection{Visuotactile Attention Visualization}

To gain further insight into the information being learned by our model, we visualize the attention weights in the latent vector cross-attention step of the transformer visuotactile encoder. For each modality, we plot attention weights as proportions of total attention to tokens in that specific modality averaged over the 8 learned latent vectors. Figure \ref{fig:attn-vis} shows an example visualization; more examples can be found on our website.

\begin{figure}[H]
     \centering
     \includegraphics[width=1.0\columnwidth]{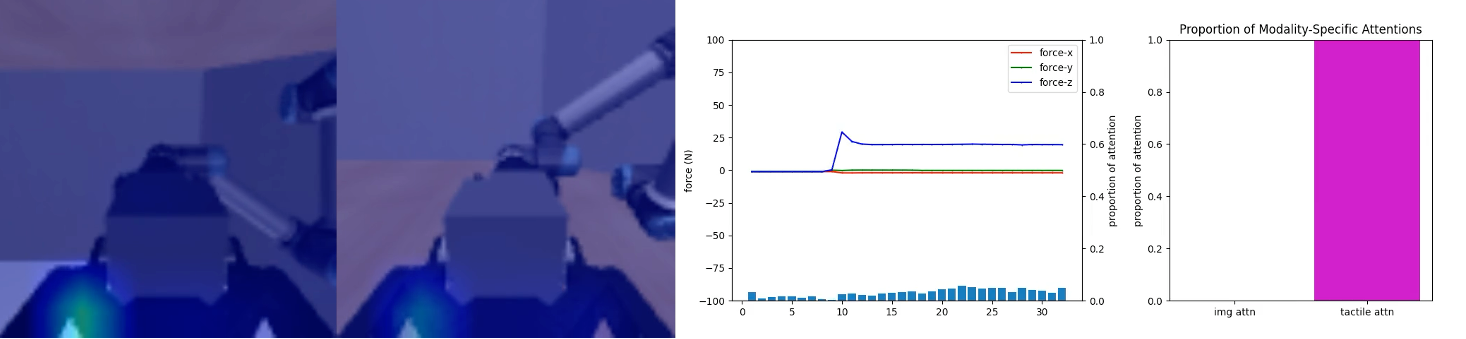}
     \caption{\footnotesize{A visualization of attention weights for vision and tactile tokens in the latent cross-attention step of the visuotactile transformer encoder. These weights are visualized as heatmaps overlayed on left and right wristview images for visual attention, and bars for each timestep under the force reading for tactile attention. We also plot the proportion of total attention for each modality (visual and tactile) during the course of a rollout.}}
     \label{fig:attn-vis}
\end{figure}

\noindent \textbf{Takeaways:} Despite our model taking in twice as many visual tokens (72 tokens, 36 per view) as tactile ones (32 tokens), we observe that tactile attention takes up almost the entire proportion of attention across the input (as seen in the right-most plot of Figure \ref{fig:attn-vis}). This finding provides further evidence to the importance of tactile information over visual information as discussed in Section \ref{sec:05E_input-modality-combinations}, where we found that removing visual information from our input had little impact on the robustness of our model. Furthermore, we observe that the visual attention is mostly focused on semantically insignficant parts of the scene, such as the gripper at the bottom of the view, suggesting that the model is not receiving much useful visual information.

\subsection{Comparing Data Augmentation Methods}

In an effort to evaluate the validity of the online augmentation method for increasing the robustness of our model, we construct a dataset of human-generated trajectories with an extended set of visual variations and sensor noise, attempting to emulate a baseline data augmentation method that applies augmentations independently to each sensory modality offline during training. More specifically, we generate a dataset with training set variations of \textit{Scene Appearance} (including object color, floor texture, and lighting), \textit{Camera Pose}, and \textit{Sensor Noise} with 12 augmentations per demonstration, but rather than keep applied variations consistent through each augmented rollout, we apply new instances of \textit{Scene Appearance} and \textit{Camera Pose} variations in each step of the demonstration. We also multiply the force and torque history reading by a random constant (from 0.1 to 2.0) independently determined each frame, following a similar data augmentation strategy used in \cite{spector2021insertionnet}. We denote this dataset as \texttt{Expanded Visual+Noise}.

We report \% success rate change from the \textit{Canonical} environment success rate on models trained on the \texttt{Expanded Visual+Noise} dataset and compare it with the training set models from our original experiment (namely \texttt{Visual+Sensor Noise} that does not apply new variation instances per frame and \texttt{Base} that includes \textit{Grasp Pose} variations); results can be found in Figure \ref{fig:extended-training-set}.

\begin{figure}[h!]
     \centering
     \includegraphics[width=1.0\columnwidth]{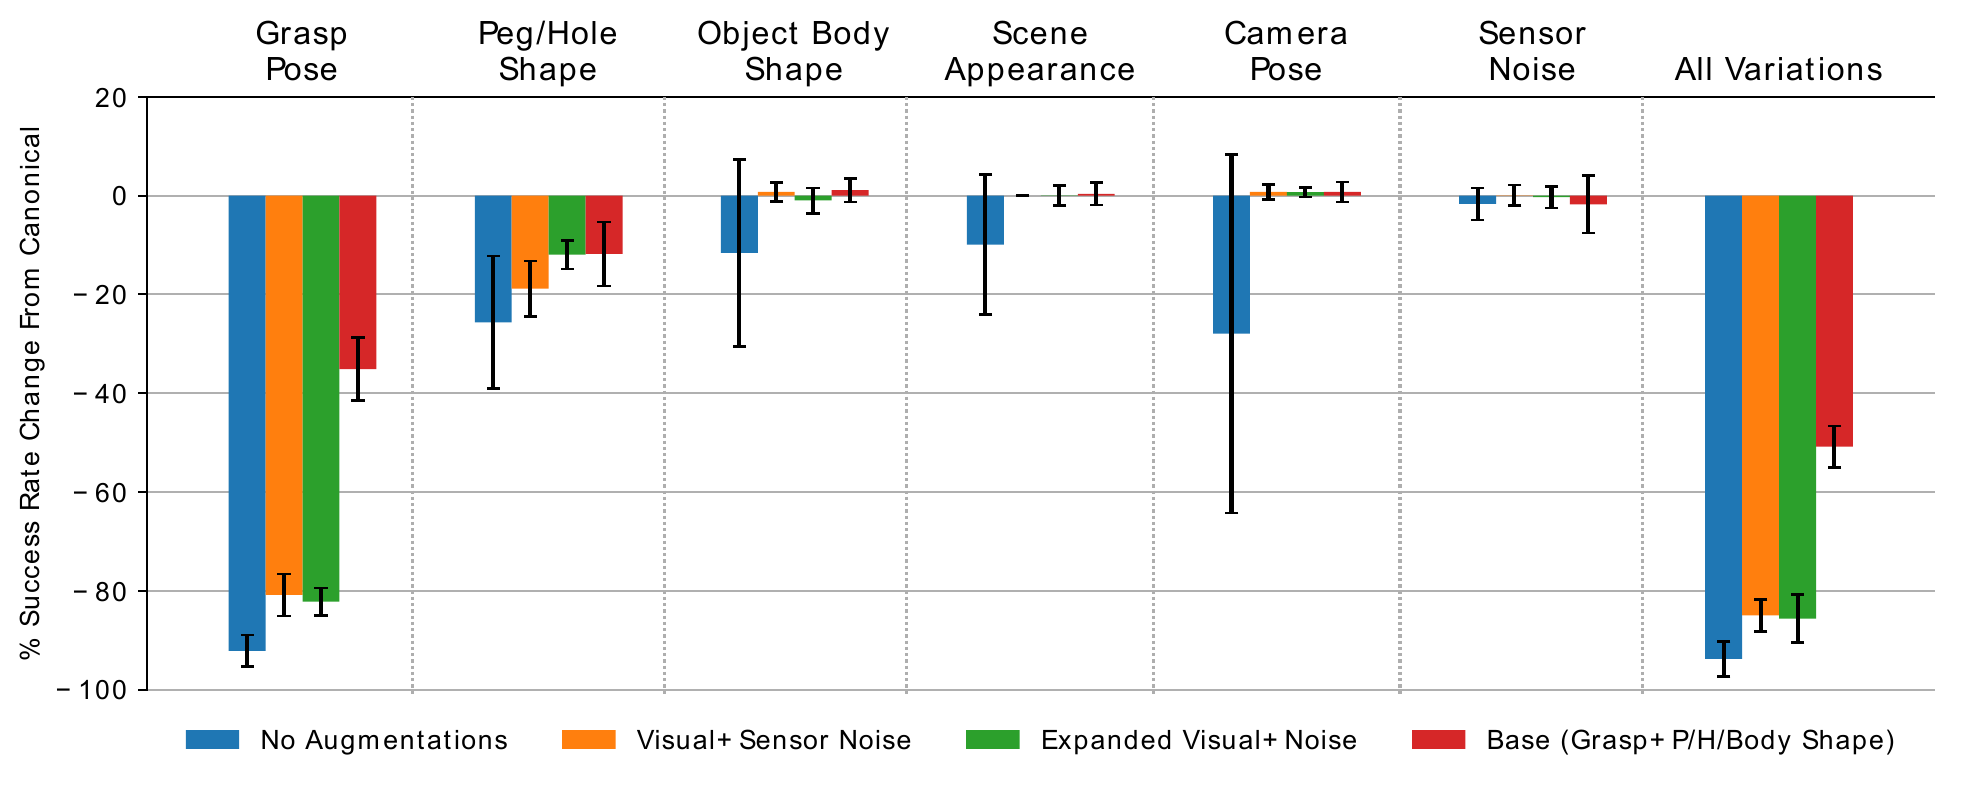}
     \caption{\footnotesize{\% success rate changes on each task variation for models trained on different subsets of task variations, including an additional \texttt{Extended Visual+Noise} dataset. Error bars represent one standard deviation from the mean. Our extended dataset of \textit{Scene Appearance}, \textit{Camera Angle}, and \textit{Sensor Noise} variations does not lead to any significant improvements on robustness to any of the task variations over the original \texttt{Visual+Sensor Noise} dataset, particularly on \textit{Grasp Pose} variations, where the inclusion of \textit{Grasp Pose} in the training dataset via online augmentation still provides the largest boost in generalization ability.}}
     \label{fig:extended-training-set}
\end{figure}

\noindent \textbf{Takeaways:} We observe that our dataset with an expanded set of augmentations independently applied to each sensory modality does not necessarily improve robustness on most task variations (save for \textit{Peg/Hole Shape}) compared to the original \texttt{Visual+Sensor Noise} dataset that was less extensive in terms of data augmentation. Most crucially, we do not see a significant improvement on \textit{Grasp Pose} variations, validating the effect of non-independent multisensory data augmentation via trajectory replay. Thus, we have shown that even extensive independent augmentation of our multisensory input may not be enough to deal with certain task variations involved in our contact-rich task.

\subsection{Success Rates for Canonical Environment}

For full transparency for our experiments that involve reporting the \% success rate change from the \textit{Canonical} environment, we explicitly report the success rates in the no-variation \textit{Canonical} environment, which the \% success rate change is based off of, for each trained model. Average success rates over 6 training seeds are reported in Figures \ref{fig:training-set-canonical-graph} and \ref{fig:modality-input-canonical-graph}. It is worth noting that the average \% success rate change across the 6 training seeds was calculated by determining the \% success rate change for each individual seed and then calculating the average over those values, rather than calculating the average success rate across the 6 seeds first and then determining the difference of those averages.

\begin{figure}[h!]
     \centering
     \includegraphics[width=0.95\columnwidth]{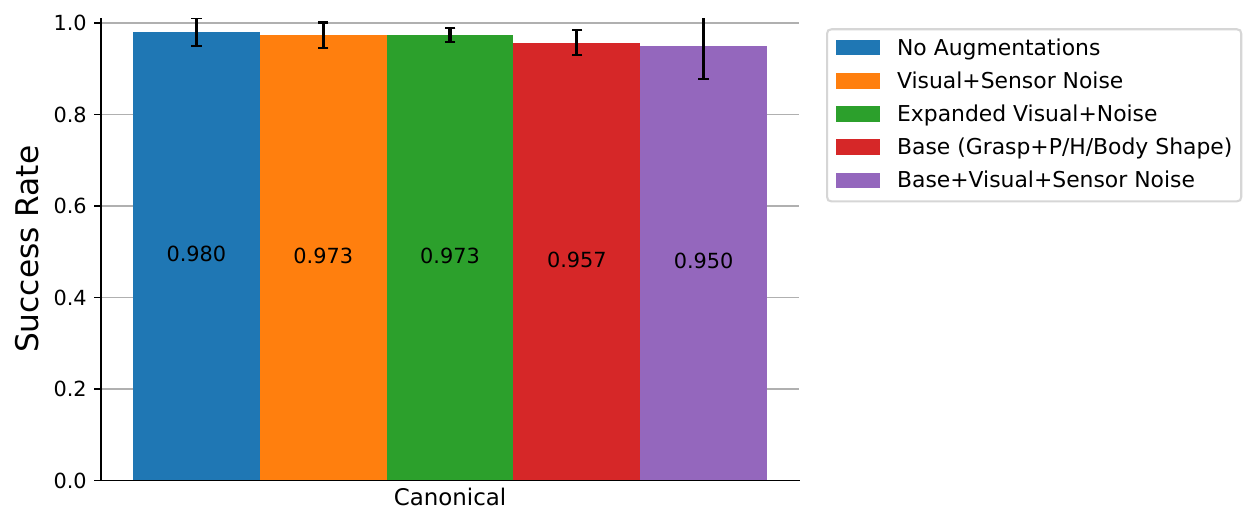}
     \caption{\footnotesize{Success rates on the \textit{Canonical} environment for models trained on different training set variations. Error bars represent one standard deviation from the mean. These success rates correspond to the results reported in Figures \ref{fig:training-set-evals} and 
     \ref{fig:extended-training-set}.}}
     \label{fig:training-set-canonical-graph}
\end{figure}

\begin{figure}[h!]
     \centering
     \includegraphics[width=0.95\columnwidth]{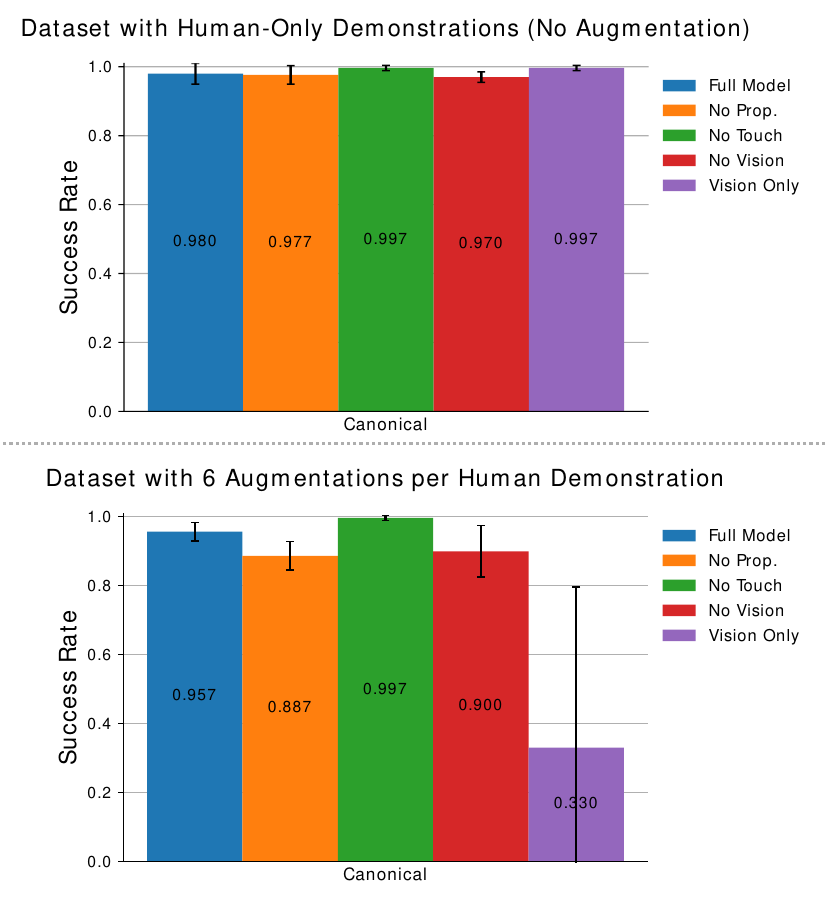}
     \caption{\footnotesize{Success rates on the \textit{Canonical} environment for models using different modality combinations as input, trained on both human-only demonstration data as well as demonstration data augmented with \textit{Grasp Pose}, \textit{Peg/Hole Shape}, and \textit{Object Body Shape} variations (denoted as the \texttt{Base} training set variations). Error bars represent one standard deviation from the mean. These success rates correspond to the results reported in Figure \ref{fig:modality-input-ablation}. We especially note the performance instability of the \texttt{No Vision} model trained on the \texttt{Base} training set variations, providing context for its omission in Figure \ref{fig:modality-input-ablation}.}}
     \label{fig:modality-input-canonical-graph}
\end{figure}

\subsection{Real-World Experimental Setup}

Our real-world task setup, shown in Figure \ref{fig:real-world-setup}, is built to mirror our simulation setup as closely as possible. We designate one arm to be compliant, applying a constant amount of force while the other arm moves according to the actions given to it by the policy. In contrast to policies trained in simulation, our real-world policies predict 2-dimensional delta actions in the axes perpendicular to the axis of insertion (rather than 3-dimensional actions that include the axis along the direction of insertion), in order to prevent potentially unsafe interactions that may occur as a result of a premature insertion attempt. Once the peg and hole are aligned, the compliant arm automatically moves its held object forward to complete the insertion.

\begin{figure}[h!]
     \centering
     \includegraphics[width=0.7\columnwidth]{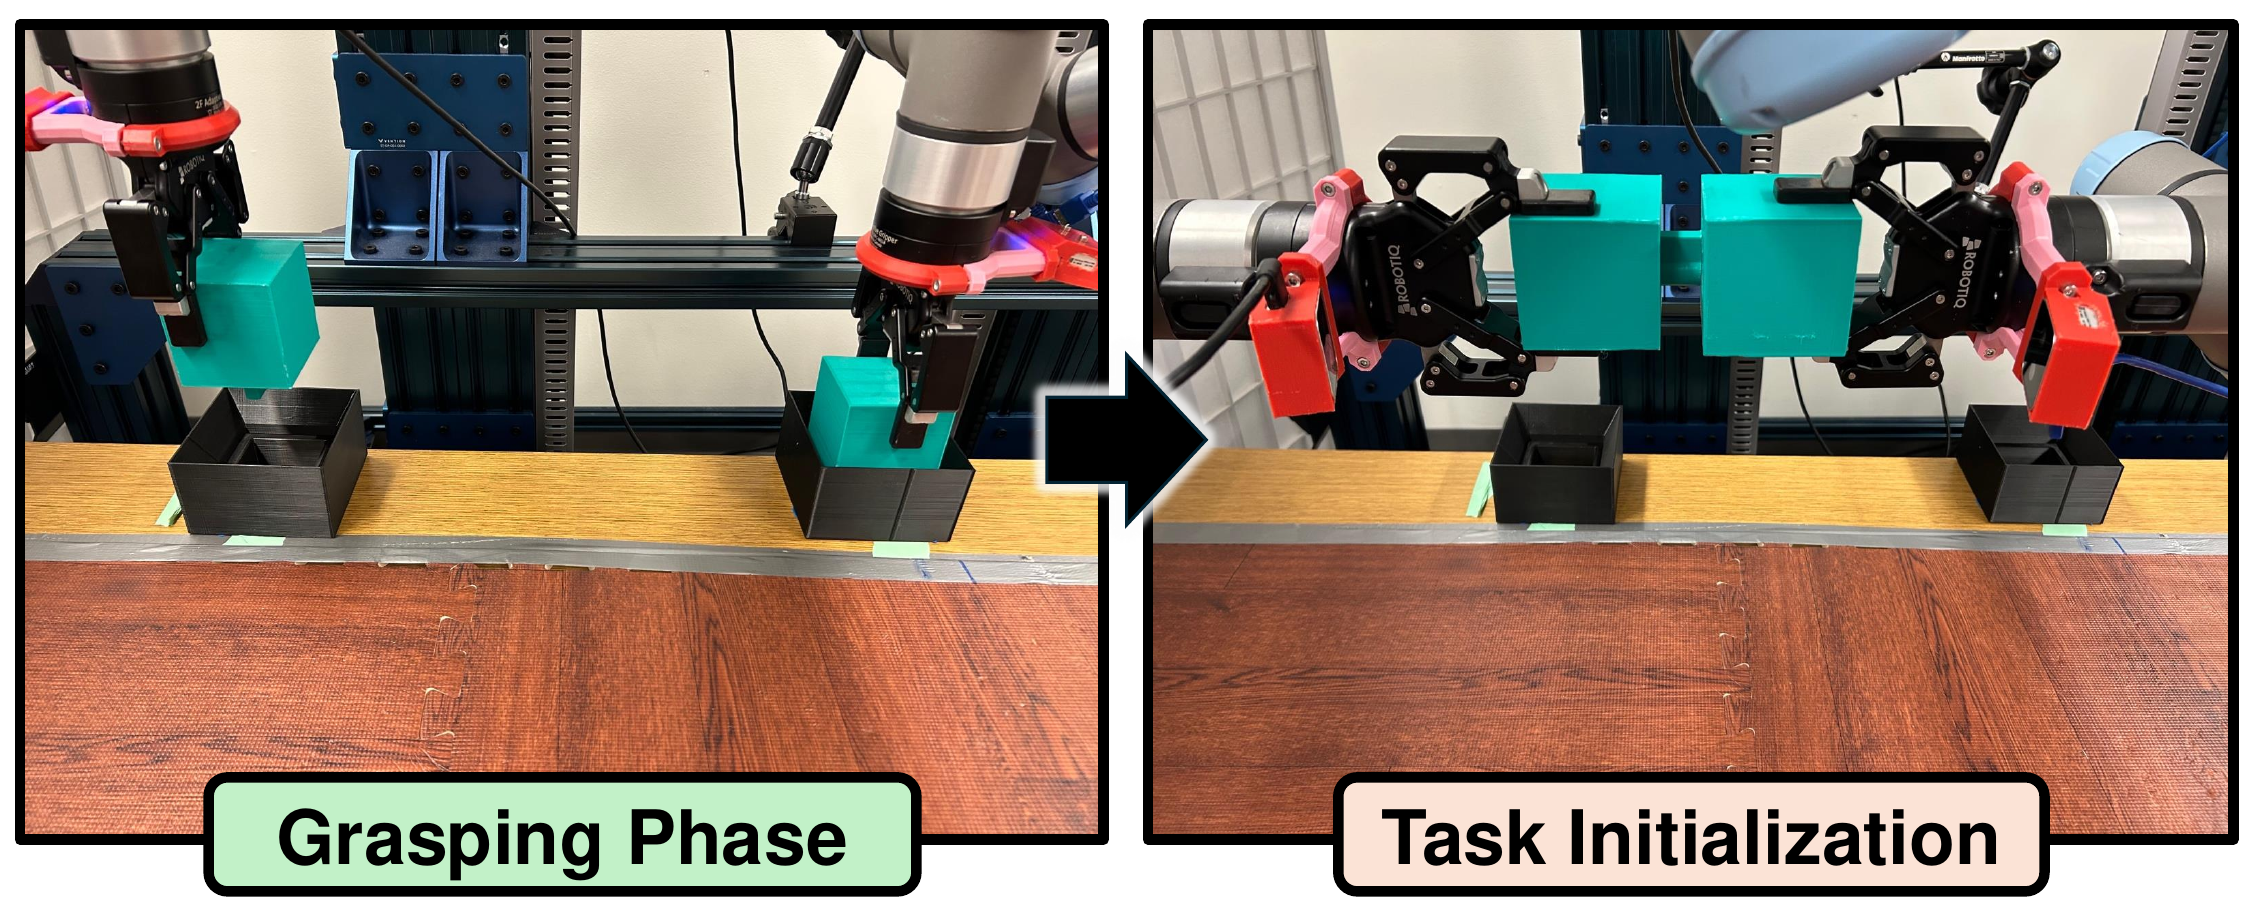}
     \caption{\footnotesize{Our real-world experimental setup. Peg and hole object models are 3D-printed directly from the model files used in our simulation environment.}}
     \label{fig:real-world-setup}
\end{figure}

We train our real-world models with the same hyperparameters as those in simulation, although we only initiate 1 training seed per model (rather than 6). Additionally, we evaluate each model at the end of the entire training process, rather than performing training set rollouts during the training process to determine the best checkpoint. Success rates are determined by the number of successful trials over 20 rollouts. Successes and failures follow the same general criteria as in simulation, though a human manually annotates successes and failures per trial.

\subsection{Real-World Experiments and Results}

\textbf{Task Variation Difficulty:} As a real-world analog to our experiments in Section \ref{sec:05A_task-variation-difficulty}, we evaluate a real-world policy trained on a dataset of human-generated demonstrations with no applied task variations on real-world versions of a subset of our task variations. Reported success rates over 20 rollouts can be found in Figure \ref{fig:real-world-canonical}.

\begin{figure}[h!]
     \centering
     \includegraphics[width=1.0\columnwidth]{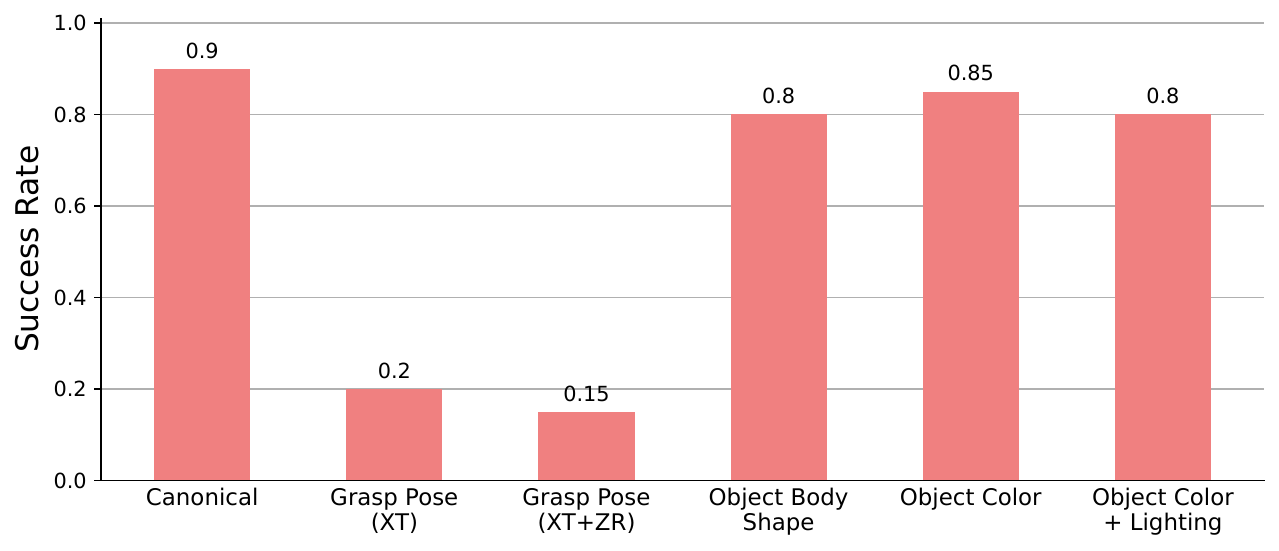}
     \caption{\footnotesize{Success rates on real-world task variations for a model trained on real-world non-augmented human demonstration data. The real-world model struggles the most with \textit{Grasp Pose} (both translation-only and translation with rotation) variations, aligning with our observations in simulation.}}
     \label{fig:real-world-canonical}
\end{figure}

\noindent \textbf{Takeaways:} Like in simulation, we observe that \textit{Grasp Pose} variations seem to be the most difficult to generalize to, while the model is able to handle the mostly unisensory perturbations of \textit{Object Body Shape} and \textit{Scene Appearance} (object color and lighting). We also notice that our model struggles with \textit{Grasp Pose} even when rotational grasp variations are removed; we hypothesize that this may be because a translational offset disrupts the desired behavior of lining up end-effector positions (given from proprioceptive input) in order to line up the peg and hole (i.e. solving the task can no longer be done by just matching the end-effector positions of the two arms). From these results, We believe that including \textit{Grasp Pose} variations into the training dataset (as was done in simulation through online augmentation) may also improve performance in the real world.

\textbf{Modality Input Ablation Study:} We conduct a reduced real-world analog to the ablation study in Section \ref{sec:05E_input-modality-combinations}. We train real-world policies on a dataset of only human demonstrations and evaluate them on a smaller subset of our real-world task variations. Reported success rates over 20 rollouts can be found in Figure \ref{fig:real-world-modality-input-ablation}.

\begin{figure}[h!]
     \centering
     \includegraphics[width=1.0\columnwidth]{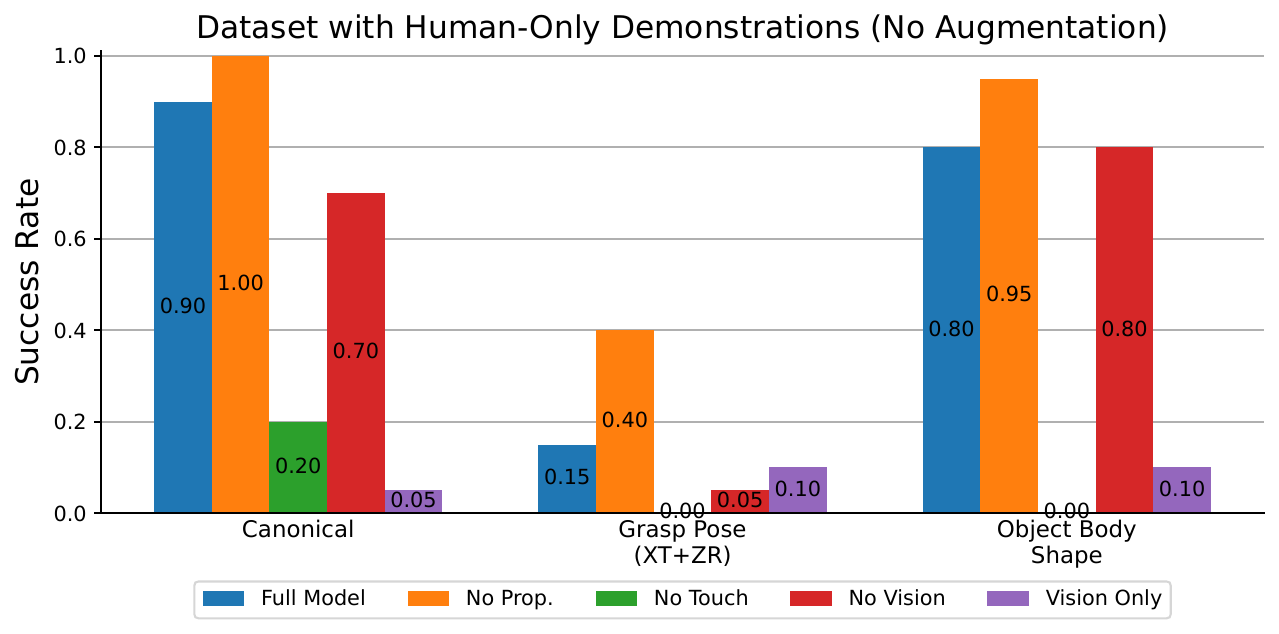}
     \caption{\footnotesize{Success rates on real-world task variations for models with different modality input combinations trained on no variations. The \texttt{No Touch} model sees the lowest success rates on all task variations, while the \texttt{No Prop.} model surprisingly sees an increase in performance over the \texttt{Full Model} for all task variations.}}
     \label{fig:real-world-modality-input-ablation}
\end{figure}

\noindent \textbf{Takeaways:} Like in simulation, we observe that the removal of force-torque data as input (the \texttt{No Touch} model) leads to a significant drop in success rate for all task variations compared to the \texttt{Full Model}, including the no-variations \textit{Canonical} environment. We also see a small drop in performance for the \texttt{No Vision} model, somewhat aligning with our findings in simulation of the insignificance of visual input for our task. Surprisingly, we see performance increases in all task variations for the \texttt{No Prop.} model. We hypothesize that the small ranges of possible end-effector poses in our training dataset due to the high precision required for our task may cause our models to not learn much useful information from the proprioceptive embedding, though this observation may of course also be the result of a low sample size of trained models. Averaging the performance of models trained over multiple seeds (as was done in simulation), which was not able to be performed due to time constraints, may give us some more robust results.
